# Supplementary material for: Deep Learning for Effective and Efficient Reduction of Large Adaptation Spaces in Self-Adaptive Systems
Source: arXiv:2204.06254 source file (2022-04-13)
Supplement: Supplementary file 1 [file appendix.tex]

\section{Grid search results}
\genidea{Add table of the grid search results for both evaluation cases}
